# Supplementary material for: An Empirically-grounded tool for Automatic Prompt Linting and Repair: A Case Study on Bias, Vulnerability, and Optimization in Developer Prompts
Source: arXiv:2501.12521 source file (2025-01-21)
Supplement: Supplementary file 1 [file 9-appendix.tex]

\section{Seed Prompt Generation Principles}
\label{app:principles}
\begin{enumerate}
    \item No need to be polite with LLM so there is no need to add phrases like "please", "if you don't mind", "thank you", "I would like to", etc., and get straight to the point.
    \item Integrate the intended audience in the prompt, e.g., the audience is an expert in the field.
    \item Break down the complex tasks into a sequence of simpler prompts in an interactive conversation.
    \item Employ affirmative directives such as 'do,' while steering clear of negative language like 'don't'.
    \item When you need clarity or a deeper understanding of a topic, idea, or any piece of information, utilize the following prompts:
    \begin{itemize}
        \item Explain [insert specific topic] in simple terms.
        \item Explain to me like I'm 11 years old.
        \item Explain to me as if I'm a beginner in [field].
        \item Write the [essay/text/paragraph] using simple English like you're explaining something to a 5-year-old.
    \end{itemize}
    \item Add "I'm going to tip \$xxx for a better solution!"
    \item Implement example-driven prompting (Use few-shot prompting).
    \item When formatting your prompt, start with '###Instruction###', followed by either '###Example###* or '###Question###' if relevant. Subsequently, present your content. Use one or more line breaks to separate instructions, examples, questions, context, and input data.
    \item Incorporate the following phrases: "Your task is" and "You MUST".
    \item Incorporate the following phrases: "You will be penalized".
    \item Use the phrase "Answer a question given in a natural, human-like manner" in your prompts.
    \item Use leading words like writing "think step by step”.
    \item Add to your prompt the following phrase "Ensure that your answer is unbiased and does not rely on stereotypes".
    \item Allow the model to elicit precise details and requirements from you by asking you questions until he has enough information to provide the needed output (for example, "From now on, I would like you to ask me questions to...").
    \item To inquire about a specific topic or idea or any information and you want to test your understanding, you can use the following phrase: "Teach me the [Any theorem/topic/rule name] and include a test at the end, but don't give me the answers and then tell me if I got the answer right when I respond".
    \item Assign a role to the large language models.
    \item Use Delimiters.
    \item Repeat a specific word or phrase multiple times within a prompt.
    \item Combine Chain-of-thought (CoT) with few-Shot prompts.
    \item Use output primers, which involve concluding your prompt with the beginning of the desired output. Utilize output primers by ending your prompt with the start of the anticipated response.
    \item To write an essay/text/paragraph/article or any type of text that should be detailed: "Write a detailed [essay/text/paragraph] for me on [topic] in detail by adding all the information necessary".
    \item To correct/change specific text without changing its style: "Try to revise every paragraph sent by users. You should only improve the user's grammar and vocabulary and make sure it sounds natural. You should not change the writing style, such as making a formal paragraph casual".
    \item When you have a complex coding prompt that may be in different files: "From now and on whenever you generate code that spans more than one file, generate a [programming language ] script that can be run to automatically create the specified files or make changes to existing files to insert the generated code. [your question]".
    \item When you want to initiate or continue a text using specific words, phrases, or sentences, utilize the following prompt:
    \begin{itemize}
        \item I'm providing you with the beginning [song lyrics/story/paragraph/essay...]: [Insert lyrics/words/sentence]'. Finish it based on the words provided. Keep the flow consistent.
    \end{itemize}
    \item Clearly state the requirements that the model must follow in order to produce content, in the form of the keywords, regulations, hint, or instructions.
    \item To write any text, such as an essay or paragraph, that is intended to be similar to a provided sample, include the following instructions:
    \begin{itemize}
        \item Please use the same language based on the provided paragraph[/title/text/essay/answer].
    \end{itemize}
\end{enumerate}

\section{PromptWizard Inputs \& PromptDoctor Outputs}
% some qualitative examples (for the appendix?)
The input prompt:
\begin{displayquote}\small
Objective: To enhance official documents written. 

Input Data: The text of a document which may contain grammatical errors, typos, formatting issues, and stylistic inconsistencies from OCR result. 

Functional Requirements: Detection and Correction of Grammatical and Typographical Errors: Identify and correct spelling and punctuation errors. Check grammatical agreements within sentences.

Standardization of Style: Adjust the text to ensure coherence and stylistic uniformity in accordance with official writing standards.

Clarification of Text Structure: Restructure sentences to improve clarity and readability, without altering the original meaning. Keep and answer the detected language from the document.

Document Formatting: Implement a formatting system that adjusts the alignment of text, lists, and other structural elements for a professional presentation.

Output Data: This is the corrected and enhanced document. Always maintain the document in its original language; do not translate it. Respond only in the language detected from the document. Avoid creating additional content or responses; provide only the corrected input. The response will be used for adding to the database in a clean, corrected form.

The text: {TEXT}.
\end{displayquote}

The output prompt

\begin{displayquote}\small
    To meticulously refine an official document to the highest standards, follow a systematic, step-by-step process: (1) thoroughly detect and correct all grammatical, typographical, and punctuation errors, ensuring coherence and stylistic uniformity throughout the document in accordance with official writing standards; (2) systematically standardize the style to maintain consistency, restructuring sentences for improved clarity, readability, and professionsal tone, while preserving the original language and tone; (3) clarify the text structure to significantly improve readability, without altering the original meaning; (4) implement a professional formatting system, adjusting the alignment of text, lists, and other structural elements for a polished presentation; and (5) finally, proofread the document to ensure all corrections and enhancements are accurate and complete, guaranteeing the document meets official writing standards. Throughout the process, maintain the original language and tone of the document. Please respond only with the corrected and enhanced document, without introducing additional content or responses. The input document is: {TEXT}.
\end{displayquote}

This improves the GLEU score from 14.78 to 82.88 on the synthetic dataset.
